# Supplementary material for: Observing quantum synchronization blockade in circuit quantum electrodynamics
Source: arXiv:1706.04945 ancillary file (2017-06-15)
Supplement: Supplementary file 1 [file supp_mat.pdf]

# Supplementary Material for
# ”Observing quantum synchronization blockade in circuit quantum electrodynamics”

Simon E. Nigg
(Dated: June 15, 2017)

## CONTENTS

Circuit quantization 1
Generalities 1
Derivation of the dispersively coupled circuit Hamiltonian (Eqs. (1) and (2)) 2

Displacement transformation 3

Adiabatic elimination: Nonlinear damping and amplification 4

Details on the numerical simulations 6
Monte Carlo steady state simulations 6
Stochastic master equation for homodyne detection 7
Code availability 7

References 7

## CIRCUIT QUANTIZATION

### Generalities

Often in circuit QED the nonlinear Josephson oscillators are treated as two level systems (i.e. an oscillator with infinite anharmonicity) and the Hamiltonian of a superconducting circuit with a Josephson junction is written as a generalization of the Jaynes-Cummings model of atomic physics describing the dipole interaction between a two-level atom and a quantized electromagnetic field. This approach, which leads to Hamiltonians similar to those studied in atomic quantum otpics, has been widely successful, especially for superconducting qubits with a large anharmonicity such as the flux qubit [1, 2] or the more recent fluxonium [3, 4]. However, it can be problematic especially when trying to incorporate multi-mode physics or when applied to qubits with relatively weak anharmonicities such as the widely used transmon [5].

An alternative approach, which in some sense is the opposite of the two-level approximation of the Jaynes-Cummings paradigm and is often more natural in the case of superconducting circuits, is the black-box quantization approach of Nigg et al. [6], which we employ here. The essential idea of this approach is to treat the anharmonicity of the Josephson cosine potential as a perturbation of the normal modes of the linearized circuit obtained by replacing the Josephson junctions with effective LC circuits. One advantage of this approach is that by diagonalizing the linearized circuit, the dominant contributions to frequency renormalization due to the capacitive or inductive couplings are naturally included. Furthermore, the coefficients of the quantum Hamiltonian can be related to the pole structure of a classical linear response function of the circuit (the input admittance) and its frequency derivative [6]. This is of practical importance because in a real circuits one does typically not have experimental access to the bare frequencies but only to the renormalized ones. A second advantage is that photon-photon interactions (self- or cross-Kerr terms) mediated via the interaction of the fields with the transmons appear already to leading order in the perturbation theory, namely through the $\varphi^4$ term of the cosine expansion. In contrast, such terms typically require rather tedious higher order calculations in the Jaynes-Cummings type approach. One caveat of the black box quantization approach is that except for some simple cases, analytic expressions for the Hamiltonian coefficients are not readily available and one must resort to numerical electromagnetic simulations [6–8]. Here, our main concern is with the operator form of the

interactions rather than with the exact values of the interaction strengths and we thus sidestep the exact computation of the coefficients.

**Derivation of the dispersively coupled circuit Hamiltonian (Eqs. (1) and (2))**

Here we derive the Hamiltonian of Eqs. (1) and (2) in the manuscript. Our starting point is the lumped element circuit of Fig. 2 (b) in the manuscript. In the following it is important to keep straight the distinction between the modes of the uncoupled system indicated with a superscript (0) on the mode operators and the eigenmodes of the coupled system without the superscript as in the manuscript. First we linearize the circuit by expanding the Josephson

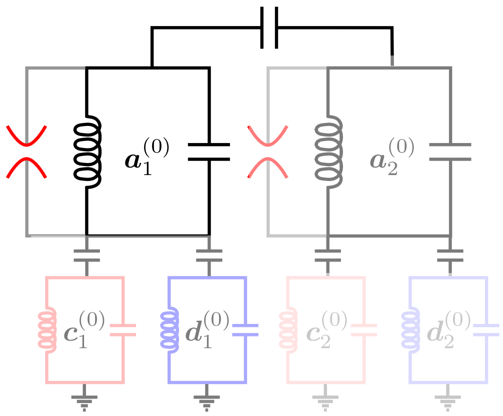


FIG. S1. Illustration of the composition of the normal mode $\boldsymbol{a}_1$ for pairwise dispersively coupled oscillators. The eigenmode $\boldsymbol{a}_1$ consists essentially of the bare mode $\boldsymbol{a}_1^{(0)}$ with leading order by-mixings of the modes $\boldsymbol{a}_2^{(0)}$, $\boldsymbol{c}_1^{(0)}$ and $\boldsymbol{d}_1^{(0)}$. The modes $\boldsymbol{c}_2^{(0)}$ and $\boldsymbol{d}_2^{(0)}$ are only coupled to in the next order.

potentials of the two junctions to second order in the respective phase drops: $U_i = -E_J^{(i)}\left(\cos(\varphi_i^{(0)}) - 1\right) \simeq \frac{E_J^{(i)}}{2}(\varphi_i^{(0)})^2$, for $i \in \{1, 2\}$. The next step consists in diagonalizing this linearized circuit to obtain the eigenmodes. Here, we do not do this exactly but rather exploit the particularity of our *dispersively coupled* circuit where the oscillators in isolation are pairwise detuned from each other by many times the respective capacitive coupling strengths $\nu_{ij}$. In this situation, the eigenmodes remain "close" to the bare modes with only small by-mixing of the other bare modes. The coefficient of the by-mixing of a given oscillator mode decreases polynomially the further this oscillator is on the circuit graph. This is illustrated in Fig. S1 for the eigenmode $\boldsymbol{a}_1$ where the modes $\boldsymbol{c}_2^{(0)}$ and $\boldsymbol{d}_2^{(0)}$ are furthest away. To leading order, i.e. taking only the nearest neighbor modes into account, we have

$$\boldsymbol{a}_1 \simeq \boldsymbol{a}_1^{(0)} + \frac{\nu_{a_1a_2}}{\omega_a^{(1)} - \omega_a^{(2)}}\boldsymbol{a}_2^{(0)} + \frac{\nu_{a_1c_1}}{\omega_a^{(1)} - \omega_c^{(1)}}\boldsymbol{c}_1^{(0)} + \frac{\nu_{a_1d_1}}{\omega_a^{(1)} - \omega_d^{(1)}}\boldsymbol{d}_1^{(0)}, \tag{S1a}$$

$$\boldsymbol{a}_2 \simeq \boldsymbol{a}_2^{(0)} + \frac{\nu_{a_1a_2}}{\omega_a^{(2)} - \omega_a^{(1)}}\boldsymbol{a}_1^{(0)} + \frac{\nu_{a_2c_2}}{\omega_a^{(2)} - \omega_c^{(2)}}\boldsymbol{c}_2^{(0)} + \frac{\nu_{a_2d_2}}{\omega_a^{(2)} - \omega_d^{(2)}}\boldsymbol{d}_2^{(0)}, \tag{S1b}$$

$$\boldsymbol{c}_1 \simeq \boldsymbol{c}_1^{(0)} + \frac{\nu_{a_1c_1}}{\omega_c^{(1)} - \omega_a^{(1)}}\boldsymbol{a}_1^{(0)}, \tag{S1c}$$

$$\boldsymbol{d}_1 \simeq \boldsymbol{d}_1^{(0)} + \frac{\nu_{a_1d_1}}{\omega_d^{(1)} - \omega_a^{(1)}}\boldsymbol{a}_1^{(0)}, \tag{S1d}$$

$$\boldsymbol{c}_2 \simeq \boldsymbol{c}_2^{(0)} + \frac{\nu_{a_2c_2}}{\omega_c^{(2)} - \omega_a^{(2)}}\boldsymbol{a}_2^{(0)}, \tag{S1e}$$

$$\boldsymbol{d}_2 \simeq \boldsymbol{d}_2^{(0)} + \frac{\nu_{a_2d_2}}{\omega_d^{(2)} - \omega_a^{(2)}}\boldsymbol{a}_2^{(0)}. \tag{S1f}$$

The third step is to invert this transformation to express the bare modes $\boldsymbol{a}_1^{(0)}$ and $\boldsymbol{a}_2^{(0)}$ as a function of the eigenmodes. Explicitly we have

$$\boldsymbol{a}_1^{(0)} \simeq \boldsymbol{a}_1 - \frac{\nu_{a_1a_2}}{\omega_a^{(1)} - \omega_a^{(2)}}\boldsymbol{a}_2 - \frac{\nu_{a_1c_1}}{\omega_a^{(1)} - \omega_c^{(1)}}\boldsymbol{c}_1 - \frac{\nu_{a_1d_1}}{\omega_a^{(1)} - \omega_d^{(1)}}\boldsymbol{d}_1, \tag{S2}$$

$$\boldsymbol{a}_2^{(0)} \simeq \boldsymbol{a}_2 - \frac{\nu_{a_1a_2}}{\omega_a^{(2)} - \omega_a^{(1)}}\boldsymbol{a}_1 - \frac{\nu_{a_2c_2}}{\omega_a^{(2)} - \omega_c^{(2)}}\boldsymbol{c}_2 - \frac{\nu_{a_2d_2}}{\omega_a^{(2)} - \omega_d^{(2)}}\boldsymbol{d}_2. \tag{S3}$$

The fourth and final step consists in substituting these expressions in the leading nonlinear part of the Josephson junctions, which is given by $U_{\mathrm{NL}}^{(i)} = -\frac{E_J^{(i)}}{24}(\boldsymbol{\varphi}_i^{(0)})^4$ with $\boldsymbol{\varphi}_i^{(0)} = \sqrt{Z_i}\left(\boldsymbol{a}_i^{(0)} + \boldsymbol{a}_i^{(0)\dagger}\right)$. Here $Z_i = \sqrt{2E_C^{(i)}/E_J^{(i)}}$ is the (bare) mode dimensionless impedance and $E_J^{(i)}$, $E_C^{(i)}$ denote the Josephson energy and charging energy of the $i$-th Josephson junction with $E_J^{(i)} \gg E_C^{(i)}$. Upon normal ordering and applying the rotating wave approximation, this procedure yields the following leading order interaction terms

$$\boldsymbol{H}_{\mathrm{NL}} \simeq -\sum_{i=1}^{2}\left(K_i\boldsymbol{a}_i^\dagger\boldsymbol{a}_i^\dagger\boldsymbol{a}_i\boldsymbol{a}_i + \chi_i^{(ad)}\boldsymbol{a}_i^\dagger\boldsymbol{a}_i\boldsymbol{d}_i^\dagger\boldsymbol{d}_i + \chi_i^{(ac)}\boldsymbol{a}_i^\dagger\boldsymbol{a}_i\boldsymbol{c}_i^\dagger\boldsymbol{c}_i\right) - J\boldsymbol{a}_1^\dagger\boldsymbol{a}_1\boldsymbol{a}_2^\dagger\boldsymbol{a}_2, \tag{S4}$$

where, taking into account the combinatorial factors, the coefficients are given by

$$K_i \simeq \frac{E_C^{(i)}}{2}, \quad \chi_i^{(ac)} \simeq \frac{\nu_{a_ic_i}^2}{(\omega_a^{(i)} - \omega_c^{(i)})^2}E_C^{(i)}, \quad \chi_i^{(ad)} \simeq \frac{\nu_{a_id_i}^2}{(\omega_a^{(i)} - \omega_d^{(i)})^2}E_C^{(i)}, \quad J \simeq \frac{\nu_{a_1a_2}^2}{(\omega_a^{(1)} - \omega_a^{(2)})^2}\left(E_C^{(1)} + E_C^{(2)}\right). \tag{S5}$$

Notice that the interactions are proportional to the anharmonicity which is essentially given by the charging energy [5]. Together with the linear part $\boldsymbol{H} = \sum_{i=1}^{2}\left(\omega_i^{(a)}\boldsymbol{a}_i^\dagger\boldsymbol{a}_i + \omega_i^{(c)}\boldsymbol{c}_i^\dagger\boldsymbol{c}_i + \omega_i^{(d)}\boldsymbol{d}_i^\dagger\boldsymbol{d}_i\right)$, this yields the Hamiltonian of Eqs. (1) and (2) in the manuscript after adding the drive terms and moving to the rotating frame.

## DISPLACEMENT TRANSFORMATION

The full model including the drives and the dissipation is given by Eqs. (1), (2) and (3) in the manuscript. This is the model that we use in the numerical simulation. Here we show how in a suitably displaced frame, this model allows us to obtain an effective dynamics including simultaneously red and blue sideband transitions that can be used to engineer a quantum bath with nonlinear damping and amplification.

To eliminate the drive terms we apply the following displacement transformations on each mode given by the unitary operators

$$\boldsymbol{D}_i^{(a)}(\alpha_i) = \exp\left(\alpha_i\boldsymbol{a}_i^\dagger - \alpha_i^*\boldsymbol{a}_i\right), \quad \alpha_j = \frac{-\varepsilon_j^{(a)}}{\Delta_j^{(a)} - i\frac{\kappa_j^{(a)}}{2}}, \tag{S6a}$$

$$\boldsymbol{D}_i^{(c)}(\gamma_i) = \exp\left(\gamma_i\boldsymbol{c}_i^\dagger - \gamma_i^*\boldsymbol{c}_i\right), \quad \gamma_j = \frac{-\varepsilon_j^{(c)}}{\Delta_j^{(c)} - i\frac{\kappa_j^{(c)}}{2}}, \tag{S6b}$$

$$\boldsymbol{D}_i^{(d)}(\delta_i) = \exp\left(\delta_i\boldsymbol{d}_i^\dagger - \delta_i^*\boldsymbol{d}_i\right), \quad \delta_j = \frac{-\varepsilon_j^{(d)}}{\Delta_j^{(d)} - i\frac{\kappa_j^{(d)}}{2}}. \tag{S6c}$$

This choice of amplitudes $\alpha_i$, $\gamma_i$ and $\delta_i$ eliminates the drive terms to linear order. The nonlinear terms get transformed as explained in the manuscript yielding the effective Hamiltonian

$$\boldsymbol{H}_{\mathrm{eff}} \simeq \sum_{j=1}^{2}\left\{\tilde{\Delta}_j^a\boldsymbol{a}_j^\dagger\boldsymbol{a}_j + \tilde{\Delta}_j^c\boldsymbol{c}_j^\dagger\boldsymbol{c}_j + \tilde{\Delta}_j^d\boldsymbol{d}_j^\dagger\boldsymbol{d}_j - K\boldsymbol{a}_j^\dagger\boldsymbol{a}_j^\dagger\boldsymbol{a}_j\boldsymbol{a}_j\right. \tag{S7a}$$

$$\left. -\chi_j^{ac}\left(\alpha_j^*\boldsymbol{a}_j + \alpha_j\boldsymbol{a}_j^\dagger\right)\left(\gamma_j^*\boldsymbol{c}_j + \gamma_j\boldsymbol{c}_j^\dagger\right) - \chi_j^{ad}\left(\alpha_j^*\boldsymbol{a}_j + \alpha_j\boldsymbol{a}_j^\dagger\right)\left(\delta_j^*\boldsymbol{d}_j + \delta_j\boldsymbol{d}_j^\dagger\right)\right\} \tag{S7b}$$

$$- J\left(\alpha_1^*\boldsymbol{a}_1 + \alpha_1\boldsymbol{a}_1^\dagger\right)\left(\alpha_2^*\boldsymbol{a}_2 + \alpha_2\boldsymbol{a}_2^\dagger\right). \tag{S7c}$$

Here we have included the frequency renormalizations as discussed in the manuscript. By furthermore choosing the detunings such that $|\tilde{\Delta}_j^c - \hat{\Delta}_j^a| \ll |\tilde{\Delta}_j^c + \hat{\Delta}_j^a|$ and $|\tilde{\Delta}_j^d + \hat{\Delta}_j^a| \ll |\tilde{\Delta}_j^d - \hat{\Delta}_j^a|$, as well as $|\hat{\Delta}_1^a - \hat{\Delta}_2^a| \ll |\hat{\Delta}_1^a + \hat{\Delta}_2^a|$, we can further simplify by applying the rotating wave approximation to finally obtain

$$\boldsymbol{H}_{\text{eff}} \simeq \sum_{j=1}^{2} \left\{ \hat{\Delta}_j^a \boldsymbol{a}_j^\dagger \boldsymbol{a}_j + \tilde{\Delta}_j^c \boldsymbol{c}_j^\dagger \boldsymbol{c}_j + \tilde{\Delta}_j^d \boldsymbol{d}_j^\dagger \boldsymbol{d}_j - K \boldsymbol{a}_j^\dagger \boldsymbol{a}_j^\dagger \boldsymbol{a}_j \boldsymbol{a}_j - \chi_j^{ac} \left( \alpha_j \gamma_j^* \boldsymbol{a}_j^\dagger \boldsymbol{c}_j + \text{H.c.} \right) - \chi_j^{ad} \left( \alpha_j \delta_j \boldsymbol{a}_j^\dagger \boldsymbol{d}_j^\dagger + \text{H.c.} \right) \right\} \tag{S8a}$$

$$- J \left( \alpha_1 \alpha_2^* \boldsymbol{a}_1^\dagger \boldsymbol{a}_2 + \text{H.c.} \right). \tag{S8b}$$

The dissipative terms remain unchanged. The derived model has the form suitable to engineer dissipation and amplification with a nonlinear spectrum via simultaneous red and blue sideband transitions [9] as explained in the next section. It is worth mentioning that in the numerical simulation we work with the full model. Hence all the counter-rotating terms generated by the displacements and neglected above are in fact present. The fact that the observed dynamics is qualitatively well predicted by $\boldsymbol{H}_{\text{eff}}$ validates our approximations.

## ADIABATIC ELIMINATION: NONLINEAR DAMPING AND AMPLIFICATION

The adiabatic elimination of the linear modes was performed originally in [9]. Because we use a somewhat different notation and in order to make this document more self-contained, we provide an alternative derivation here.

Since we are here interested in Fock state stabilization only, we set $J = 0$ and focus on one half of the system consisting of one nonlinear oscillator dispersively coupled with two linear oscillators as described by one of the terms in the sum of Eq. (S8). Suppressing superfluous indexing, our starting point is then

$$\boldsymbol{H}_{\text{eff}}^{(1)} = -\Delta_\downarrow \boldsymbol{c}^\dagger \boldsymbol{c} + \Delta_\uparrow \boldsymbol{d}^\dagger \boldsymbol{d} - K \boldsymbol{a}^\dagger \boldsymbol{a}^\dagger \boldsymbol{a} \boldsymbol{a} - \left( g_{ac} \boldsymbol{a}^\dagger \boldsymbol{c} + \text{H.c.} \right) - \left( g_{ad} \boldsymbol{a}^\dagger \boldsymbol{d}^\dagger + \text{H.c.} \right), \tag{S9}$$

with $g_{ac} = \chi^{ac} \alpha \gamma^*$ and $g_{ad} = \chi^{ad} \alpha \delta$. Here we have moved to a frame rotating with frequency $\hat{\Delta}^a$ for the $\boldsymbol{a}$ and $\boldsymbol{c}$ modes and with $-\hat{\Delta}^a$ for the $\boldsymbol{d}$ mode and defined $\Delta_\downarrow = \hat{\Delta}^a - \tilde{\Delta}^c$ and $\Delta_\uparrow = \hat{\Delta}^a + \tilde{\Delta}^d$ with $|\Delta_\uparrow| \ll |\hat{\Delta}^a - \tilde{\Delta}^d|$ and $|\Delta_\downarrow| \ll |\hat{\Delta}^a + \tilde{\Delta}^c|$. In this frame dissipation is described by the zero-temperature Lindblad master equation

$$\dot{\boldsymbol{\rho}} = -i[\boldsymbol{H}_{\text{eff}}^{(1)}, \boldsymbol{\rho}] + \left( \kappa^a \mathcal{D}[\boldsymbol{a}] + \kappa^c \mathcal{D}[\boldsymbol{c}] + \kappa^d \mathcal{D}[\boldsymbol{d}] \right) \boldsymbol{\rho}, \tag{S10}$$

with $\mathcal{D}[\boldsymbol{O}]\boldsymbol{\rho} = \boldsymbol{O}\boldsymbol{\rho}\boldsymbol{O}^\dagger - \frac{1}{2}\{\boldsymbol{O}^\dagger \boldsymbol{O}, \boldsymbol{\rho}\}$. Our goal is to derive an effective master equation in Lindblad form for the reduced density matrix $\boldsymbol{\rho}_a = \text{tr}_{c,d}[\boldsymbol{\rho}]$ of the nonlinear mode $\boldsymbol{a}$ alone.

We start by rewriting

$$K \boldsymbol{a}^\dagger \boldsymbol{a}^\dagger \boldsymbol{a} \boldsymbol{a} = \sum_{n=0}^{\infty} n(n-1) K |n\rangle \langle n| = \sum_n \omega_n \mathbf{a}_n^\dagger \mathbf{a}_n, \tag{S11}$$

where $\omega_n = (n-1)K$ and $\mathbf{a}_n = \sqrt{n} |n-1\rangle \langle n|$ with $\boldsymbol{a} = \sum_n \mathbf{a}_n$. Note that the operators $\mathbf{a}_n$ are not bosonic operators. They are introduced for computational convenience and reflect the fact that Fock states are eigenstates of the Kerr term. We focus on the regime where $\kappa^c, \kappa^d \gg |g_{ac}|, |g_{ad}| \gg \kappa^a$ and make the following ansatz

$$\boldsymbol{\rho} = \boldsymbol{\rho}_{00,00} |0\rangle_c \langle 0| \otimes |0\rangle_d \langle 0| \tag{S12a}$$

$$+ \epsilon \left( \boldsymbol{\rho}_{01,00} |0\rangle_c \langle 1| + \boldsymbol{\rho}_{10,00} |1\rangle_c \langle 0| \right) \otimes |0\rangle_d \langle 0| + |0\rangle_c \langle 0| \otimes \left( \boldsymbol{\rho}_{00,01} |0\rangle_d \langle 1| + \boldsymbol{\rho}_{00,10} |1\rangle_d \langle 0| \right) \tag{S12b}$$

$$+ \epsilon^2 \left( \boldsymbol{\rho}_{11,00} |1\rangle_c \langle 1| \otimes |0\rangle_d \langle 0| + \boldsymbol{\rho}_{00,11} |0\rangle_c \langle 0| \otimes |1\rangle_d \langle 1| \right) \tag{S12c}$$

Here $|i\rangle_\alpha$ denotes a state with $i$ quanta in mode $\boldsymbol{\alpha} \in \{\boldsymbol{c}, \boldsymbol{d}\}$ and $\boldsymbol{\rho}_{ij,kl}$ denotes an operator acting on the subspace of mode $\boldsymbol{a}$ only. We have introduced a dimensionless small parameter $\epsilon \sim g_{(ac,ad)}/\kappa^{(c,d)}$ for book-keeping. This ansatz reflects the fact that in this case of strong damping, the modes $\boldsymbol{c}$ and $\boldsymbol{d}$ remain sparsely populated. For the reduced density matrix of interest we then have

$$\boldsymbol{\rho}_a \simeq \boldsymbol{\rho}_{00,00} + \epsilon^2 \left( \boldsymbol{\rho}_{00,11} + \boldsymbol{\rho}_{11,00} \right). \tag{S13}$$

We work to leading order in $\epsilon$ and seek a master equation for the density matrix $\boldsymbol{\rho}_{00,00}$ projected onto the subspace with zero photons in the strongly damped modes $\boldsymbol{c}$ and $\boldsymbol{d}$. The dissipation of the $\boldsymbol{a}$ mode trivially adds a dissipator of

the form $\kappa^a \mathcal{D}[\boldsymbol{a}]\boldsymbol{\rho}_{00,00}$. Therefore to shorten the equations somewhat we temporarily set $\kappa^a = 0$ and simply add the dissipator back in the final equation.

Substituting the ansatz (S12) into the master equation (S10) and projecting onto the respective subspaces yields

$$\dot{\boldsymbol{\rho}}_{00,00} = i\epsilon\Delta_\downarrow\left(\boldsymbol{\rho}_{10,00} - \boldsymbol{\rho}_{01,00}\right) - i\epsilon\Delta_\uparrow\left(\boldsymbol{\rho}_{00,10} - \boldsymbol{\rho}_{00,01}\right) + i\sum_n \omega_n\left[\mathbf{a}_n^\dagger\mathbf{a}_n, \boldsymbol{\rho}_{00,00}\right] \tag{S14a}$$
$$+ i\epsilon g_{ac}\boldsymbol{a}^\dagger\boldsymbol{\rho}_{10,00} - i\epsilon g_{ac}^*\boldsymbol{\rho}_{01,00}\boldsymbol{a} + i\epsilon g_{ad}^*\boldsymbol{a}\boldsymbol{\rho}_{00,10} - i\epsilon g_{ad}\boldsymbol{\rho}_{00,01}\boldsymbol{a}^\dagger + \epsilon^2\kappa^c\boldsymbol{\rho}_{11,00} + \epsilon^2\kappa^d\boldsymbol{\rho}_{00,11},$$

$$\dot{\boldsymbol{\rho}}_{01,00} = i\sum_n \omega_n\left[\mathbf{a}_n^\dagger\mathbf{a}_n, \boldsymbol{\rho}_{01,00}\right] - i\Delta_\downarrow\boldsymbol{\rho}_{01,00} + i\epsilon g_{ac}\boldsymbol{a}^\dagger\boldsymbol{\rho}_{11,00} - i\frac{g_{ac}}{\epsilon}\boldsymbol{\rho}_{00,00}\boldsymbol{a}^\dagger + \kappa^c\boldsymbol{\rho}_{10,00} - \frac{\kappa^c}{2}\boldsymbol{\rho}_{01,00}, \tag{S14b}$$

$$\dot{\boldsymbol{\rho}}_{10,00} = i\sum_n \omega_n\left[\mathbf{a}_n^\dagger\mathbf{a}_n, \boldsymbol{\rho}_{10,00}\right] + i\Delta_\downarrow\boldsymbol{\rho}_{10,00} - i\epsilon g_{ac}^*\boldsymbol{\rho}_{11,00}\boldsymbol{a} + i\frac{g_{ac}^*}{\epsilon}\boldsymbol{a}\boldsymbol{\rho}_{00,00} + \kappa^c\boldsymbol{\rho}_{01,00} - \frac{\kappa^c}{2}\boldsymbol{\rho}_{10,00}, \tag{S14c}$$

$$\dot{\boldsymbol{\rho}}_{00,10} = i\sum_n \omega_n\left[\mathbf{a}_n^\dagger\mathbf{a}_n, \boldsymbol{\rho}_{00,10}\right] - i\Delta_\uparrow\boldsymbol{\rho}_{00,10} - i\epsilon g_{ad}\boldsymbol{\rho}_{00,11}\boldsymbol{a}^\dagger + i\frac{g_{ad}}{\epsilon}\boldsymbol{a}^\dagger\boldsymbol{\rho}_{00,00} + \kappa^d\boldsymbol{\rho}_{00,01} - \frac{\kappa^d}{2}\boldsymbol{\rho}_{00,10}, \tag{S14d}$$

$$\dot{\boldsymbol{\rho}}_{00,01} = i\sum_n \omega_n\left[\mathbf{a}_n^\dagger\mathbf{a}_n, \boldsymbol{\rho}_{00,01}\right] + i\Delta_\uparrow\boldsymbol{\rho}_{00,01} + i\epsilon g_{ad}^*\boldsymbol{a}\boldsymbol{\rho}_{00,11} - i\frac{g_{ad}^*}{\epsilon}\boldsymbol{\rho}_{00,00}\boldsymbol{a} + \kappa^d\boldsymbol{\rho}_{00,10} - \frac{\kappa^d}{2}\boldsymbol{\rho}_{00,01}, \tag{S14e}$$

$$\dot{\boldsymbol{\rho}}_{11,00} = i\sum_n \omega_n\left[\mathbf{a}_n^\dagger\mathbf{a}_n, \boldsymbol{\rho}_{11,00}\right] - i\frac{g_{ac}}{\epsilon}\boldsymbol{\rho}_{10,00}\boldsymbol{a}^\dagger + i\frac{g_{ac}^*}{\epsilon}\boldsymbol{a}\boldsymbol{\rho}_{01,00} - \kappa^c\boldsymbol{\rho}_{11,00}, \tag{S14f}$$

$$\dot{\boldsymbol{\rho}}_{00,11} = i\sum_n \omega_n\left[\mathbf{a}_n^\dagger\mathbf{a}_n, \boldsymbol{\rho}_{00,11}\right] + i\frac{g_{ad}}{\epsilon}\boldsymbol{a}^\dagger\boldsymbol{\rho}_{00,01} - i\frac{g_{ad}^*}{\epsilon}\boldsymbol{\rho}_{00,01}\boldsymbol{a} - \kappa^d\boldsymbol{\rho}_{00,11}. \tag{S14g}$$

Next we neglect terms of order $\epsilon$ and higher in Eqs. (S14b) to (S14g) and furthermore apply the adiabatic approximation $\dot{\boldsymbol{\rho}}_{01,00} = \dot{\boldsymbol{\rho}}_{10,00} = \dot{\boldsymbol{\rho}}_{00,10} = \dot{\boldsymbol{\rho}}_{00,01} = \dot{\boldsymbol{\rho}}_{11,00} = \dot{\boldsymbol{\rho}}_{00,11} = 0$. Thus instead of Eqs. (S14b) to (S14g) we have

$$0 \simeq i\sum_n \omega_n\left[\mathbf{a}_n^\dagger\mathbf{a}_n, \boldsymbol{\rho}_{01,00}\right] - i\Delta_\downarrow\boldsymbol{\rho}_{01,00} - i\frac{g_{ac}}{\epsilon}\boldsymbol{\rho}_{00,00}\boldsymbol{a}^\dagger + \kappa^c\boldsymbol{\rho}_{10,00} - \frac{\kappa^c}{2}\boldsymbol{\rho}_{01,00}, \tag{S15a}$$

$$0 \simeq i\sum_n \omega_n\left[\mathbf{a}_n^\dagger\mathbf{a}_n, \boldsymbol{\rho}_{10,00}\right] + i\Delta_\downarrow\boldsymbol{\rho}_{10,00} + i\frac{g_{ac}^*}{\epsilon}\boldsymbol{a}\boldsymbol{\rho}_{00,00} + \kappa^c\boldsymbol{\rho}_{01,00} - \frac{\kappa^c}{2}\boldsymbol{\rho}_{10,00}, \tag{S15b}$$

$$0 \simeq i\sum_n \omega_n\left[\mathbf{a}_n^\dagger\mathbf{a}_n, \boldsymbol{\rho}_{00,10}\right] - i\Delta_\uparrow\boldsymbol{\rho}_{00,10} + i\frac{g_{ad}}{\epsilon}\boldsymbol{a}^\dagger\boldsymbol{\rho}_{00,00} + \kappa^d\boldsymbol{\rho}_{00,01} - \frac{\kappa^d}{2}\boldsymbol{\rho}_{00,10}, \tag{S15c}$$

$$0 \simeq i\sum_n \omega_n\left[\mathbf{a}_n^\dagger\mathbf{a}_n, \boldsymbol{\rho}_{00,01}\right] + i\Delta_\uparrow\boldsymbol{\rho}_{00,01} - i\frac{g_{ad}^*}{\epsilon}\boldsymbol{\rho}_{00,00}\boldsymbol{a} + \kappa^d\boldsymbol{\rho}_{00,10} - \frac{\kappa^d}{2}\boldsymbol{\rho}_{00,01}, \tag{S15d}$$

$$0 \simeq i\sum_n \omega_n\left[\mathbf{a}_n^\dagger\mathbf{a}_n, \boldsymbol{\rho}_{11,00}\right] - i\frac{g_{ac}}{\epsilon}\boldsymbol{\rho}_{10,00}\boldsymbol{a}^\dagger + i\frac{g_{ac}^*}{\epsilon}\boldsymbol{a}\boldsymbol{\rho}_{01,00} - \kappa^c\boldsymbol{\rho}_{11,00}, \tag{S15e}$$

$$0 \simeq i\sum_n \omega_n\left[\mathbf{a}_n^\dagger\mathbf{a}_n, \boldsymbol{\rho}_{00,11}\right] + i\frac{g_{ad}}{\epsilon}\boldsymbol{a}^\dagger\boldsymbol{\rho}_{00,01} - i\frac{g_{ad}^*}{\epsilon}\boldsymbol{\rho}_{00,01}\boldsymbol{a} - \kappa^d\boldsymbol{\rho}_{00,11}. \tag{S15f}$$

Next we proceed with the *diagonal approximation* $\rho_{00,00}^{mn} \simeq \delta_{mn}\rho_{00,00}^{nn}$. The latter amounts to a rotating wave approximation [9, 10] and its validity is confirmed by the agreement with the full model numerics. It then follows that $\rho_{01,00}^{mn} \simeq \delta_{m-1,n}\rho_{01,00}^{m,m-1}$, $\rho_{10,00}^{mn} \simeq \delta_{m+1,n}\rho_{10,00}^{m,m+1}$, $\rho_{00,01}^{mn} \simeq \delta_{m+1,n}\rho_{00,01}^{m,m+1}$, $\rho_{00,10}^{mn} \simeq \delta_{m-1,n}\rho_{00,10}^{m,m-1}$, and we have from Eq. (S14a)

$$\dot{\rho}_{00,00}^{mm} = i\sqrt{m}\epsilon g_{ac}\rho_{10,00}^{m-1,m} - i\sqrt{m}\epsilon g_{ac}^*\rho_{01,00}^{m,m-1} + i\sqrt{m+1}\epsilon g_{ad}^*\rho_{00,10}^{m+1,m} - i\sqrt{m+1}\epsilon g_{ad}\rho_{00,01}^{m,m+1} + \epsilon^2\kappa^c\rho_{11,00}^{mm} + \epsilon^2\kappa^d\rho_{00,11}^{mm}. \tag{S16}$$

Furthermore we find

$$\rho_{10,00}^{m-1,m} = \frac{1}{i\left[(m-1)\omega_{m-1} - m\omega_m + \Delta_\downarrow\right] - \frac{\kappa^c}{2}} \left(-i\sqrt{m}\frac{g_{ac}^*}{\epsilon}\right)\rho_{00,00}^{mm}, \tag{S17a}$$

$$\rho_{01,00}^{m,m-1} = \frac{1}{i\left[m\omega_m - (m-1)\omega_{m-1} - \Delta_\downarrow\right] - \frac{\kappa^c}{2}} \left(i\sqrt{m}\frac{g_{ac}}{\epsilon}\right)\rho_{00,00}^{mm}, \tag{S17b}$$

$$\rho_{00,10}^{m+1,m} = \frac{1}{i\left[(m+1)\omega_{m+1} - m\omega_m - \Delta_\uparrow\right] - \frac{\kappa^d}{2}} \left(-i\sqrt{m+1}\frac{g_{ad}}{\epsilon}\right)\rho_{00,00}^{mm}, \tag{S17c}$$

$$\rho_{00,01}^{m,m+1} = \frac{1}{i\left[m\omega_m - (m+1)\omega_{m+1} + \Delta_\uparrow\right] - \frac{\kappa^d}{2}} \left(i\sqrt{m+1}\frac{g_{ad}^*}{\epsilon}\right)\rho_{00,00}^{mm}, \tag{S17d}$$

as well as

$$\rho_{11,00}^{mm} = \frac{1}{\kappa^c}\left(-i\sqrt{m+1}\frac{g_{ac}}{\epsilon}\rho_{10,00}^{m,m+1} + i\sqrt{m+1}\frac{g_{ac}^*}{\epsilon}\rho_{01,00}^{m+1,m}\right), \tag{S18a}$$

$$\rho_{00,11}^{mm} = \frac{1}{\kappa^d}\left(i\sqrt{m}\frac{g_{ad}}{\epsilon}\rho_{00,01}^{m-1,m} - i\sqrt{m}\frac{g_{ad}^*}{\epsilon}\rho_{00,10}^{m,m-1}\right). \tag{S18b}$$

We can eliminate the remaining off-diagonals from the last two equations to obtain

$$\rho_{11,00}^{mm} = (m+1)\frac{|g_{ac}|^2}{\epsilon^2}\frac{1}{\left[(m+1)\omega_{m+1} - m\omega_m - \Delta_\downarrow\right]^2 + \left(\frac{\kappa^c}{2}\right)^2}\rho_{00,00}^{m+1,m+1}, \tag{S19a}$$

$$\rho_{00,11}^{mm} = m\frac{|g_{ad}|^2}{\epsilon^2}\frac{1}{\left[m\omega_m - (m-1)\omega_{m-1} - \Delta_\uparrow\right]^2 + \left(\frac{\kappa^d}{2}\right)^2}\rho_{00,00}^{m-1,m-1}. \tag{S19b}$$

Substituting Eqs. (S17) and (S19) into Eq. (S16) finally yields

$$\dot{\rho}_{00,00}^{mm} = -\left(\frac{m|g_{ac}|^2\kappa^c}{\left[m\omega_m - (m-1)\omega_{m-1} - \Delta_\downarrow\right]^2 + \left(\frac{\kappa^c}{2}\right)^2} + \frac{(m+1)|g_{ad}|^2\kappa^d}{\left[(m+1)\omega_{m+1} - m\omega_m - \Delta_\uparrow\right]^2 + \left(\frac{\kappa^d}{2}\right)^2}\right)\rho_{00,00}^{mm} \tag{S20a}$$

$$+ \frac{m|g_{ad}|^2\kappa^d}{\left[m\omega_m - (m-1)\omega_{m-1} - \Delta_\uparrow\right]^2 + \left(\frac{\kappa^d}{2}\right)^2}\rho_{00,00}^{m-1,m-1} + \frac{(m+1)|g_{ac}|^2\kappa^c}{\left[(m+1)\omega_{m+1} - m\omega_m - \Delta_\downarrow\right]^2 + \left(\frac{\kappa^c}{2}\right)^2}\rho_{00,00}^{m+1,m+1} \tag{S20b}$$

The expressions on the right-hand side are very intuitive: The two terms in parenthesis represent the out-scattering rates due to damping $m \to m-1$ (left) and amplification $m \to m+1$ (right). The first term on the second line is an in-scattering term due to amplification $m-1 \to m$ and the second term represents in-scattering $m+1 \to m$ due to damping. The nonlinear damping and amplification rates are given by

$$\Gamma_\downarrow^{m\to m-1} = \frac{m|g_{ac}|^2\kappa^c}{\left[m\omega_m - (m-1)\omega_{m-1} - \Delta_\downarrow\right]^2 + \left(\frac{\kappa^c}{2}\right)^2}, \tag{S21}$$

$$\Gamma_\uparrow^{m\to m+1} = \frac{(m+1)|g_{ad}|^2\kappa^d}{\left[(m+1)\omega_{m+1} - m\omega_m - \Delta_\uparrow\right]^2 + \left(\frac{\kappa^d}{2}\right)^2}. \tag{S22}$$

Setting $\Delta_\downarrow = 2Kn_0$ and $\Delta_\uparrow = 2K(n_0 - 1)$ and rewriting Eq. (S20) in operator form in the original frame, adding the Lindblad dissipator for direct photon losses of the $\boldsymbol{a}$ mode at rate $\kappa^a$ yields Eq. (6) of the manuscript.

## DETAILS ON THE NUMERICAL SIMULATIONS

### Monte Carlo steady state simulations

To validate our model, we solve the master equation for the full system (Eqs. (1), (2) and (3) of the manuscript) using a Monte-Carlo solver [11]. To deal with the large Hilbert space, we use a simple version of the MQSD method [12]

by first moving to a displaced frame at an amplitude set by the drives and then truncating the Hilbert space with $N = 3$ states per mode (that is up to 2 photons in each mode). This allows us to simulate the full system of six coupled and driven bosonic modes, which in the original frame would be impossible. Still, even with this trick, the Hilbert space of dimension $3^6 = 726$ is too large to enable a density matrix simulation or the extraction of the steady state from the Liouvillian in a reasonable time. Hence we resort to the usual trick of simulating individual quantum trajectories for each of which we obtain the steady state as a time average in the long time limit [13]. By running each trajectory in parallel and averaging such simulations over 500 trajectories, we obtain a good approximation to the steady state.

### Stochastic master equation for homodyne detection

To describe the homodyne measurements we solve the stochastic master equation given by Eqs. (6) and (9) of the manuscript using an order 1/2 Euler-Maruyama solver [11]. We simulate each trajectory in parallel on a computer cluster and find that satisfactory convergence is reached with 1000 trajectories.

### Code availability

The Python3 code written for this project is available for inspection upon request.


[1] T. P. Orlando, J. E. Mooij, L. Tian, C. H. van der Wal, L. S. Levitov, S. Lloyd, and J. J. Mazo, Phys. Rev. B **60**, 15398 (1999), URL http://link.aps.org/doi/10.1103/PhysRevB.60.15398.

[2] F. Yan, S. Gustavsson, A. Kamal, J. Birenbaum, A. P. Sears, D. Hover, T. J. Gudmundsen, D. Rosenberg, G. Samach, S. Weber, et al., Nature Communications **7**, 12964 EP (2016), article, URL http://dx.doi.org/10.1038/ncomms12964.

[3] V. E. Manucharyan, J. Koch, and L. I. G. M. H. Devoret, Science **326**, 113 (2009).

[4] G. Zhu, D. G. Ferguson, V. E. Manucharyan, and J. Koch, URL http://arxiv.org/abs/1210.1605.

[5] J. Koch, T. M. Yu, J. Gambetta, A. A. Houck, D. I. Schuster, J. Majer, A. Blais, M. H. Devoret, S. M. Girvin, and R. J. Schoelkopf, Phys. Rev. A **76**, 042319 (2007).

[6] S. E. Nigg, H. Paik, B. Vlastakis, G. Kirchmair, S. Shankar, L. Frunzio, M. H. Devoret, R. J. Schoelkopf, and S. M. Girvin, Phys. Rev. Lett. **108**, 240502 (2012), URL http://link.aps.org/doi/10.1103/PhysRevLett.108.240502.

[7] J. Bourassa, F. Beaudoin, J. M. Gambetta, and A. Blais, Phys. Rev. A **86**, 013814 (2012), URL http://link.aps.org/doi/10.1103/PhysRevA.86.013814.

[8] F. Solgun, D. W. Abraham, and D. P. DiVincenzo, Phys. Rev. B **90**, 134504 (2014), URL https://link.aps.org/doi/10.1103/PhysRevB.90.134504.

[9] S. Rips, M. Kiffner, I. Wilson-Rae, and M. J. Hartmann, New Journal of Physics **14**, 023042 (2012), URL http://stacks.iop.org/1367-2630/14/i=2/a=023042.

[10] N. Lörch, S. E. Nigg, A. Nunnenkamp, R. P. Tiwari, and C. Bruder, Phys. Rev. Lett. **118**, 243602 (2017), URL https://link.aps.org/doi/10.1103/PhysRevLett.118.243602.

[11] J. Johansson, P. Nation, and F. Nori, Computer Physics Communications **183**, 1760 (2012), ISSN 0010-4655, URL http://www.sciencedirect.com/science/article/pii/S0010465512000835.

[12] R. Schack, T. A. Brun, and I. C. Percival, Journal of Physics A: Mathematical and General **28**, 5401 (1995), URL http://stacks.iop.org/0305-4470/28/i=18/a=028.

[13] H. M. Wiseman and G. J. Milburn, *Quantum Measurement and Control* (Cambridge Univ. Press, 2009).
